# Supplementary material for: Cross-Domain Neural Entity Linking
Source: arXiv:2210.15616 source file (2022-09-28)
Supplement: Supplementary file 1 [file Appendix.tex]

%!TEX root = ../Thesis.tex

TBC.
